# Supplementary material for: Few-Shot Named Entity Recognition: A Comprehensive Study
Source: arXiv:2012.14978 source file (2020-12-29)
Supplement: Supplementary file 1 [file appendix.tex]

\begin{table*}[ht]
    \centering
    \small
    \begin{tabular}{c|c|c|c|c|c|c|c}
    \toprule
    Datasets & Settings & \hlightPyellow{\text{NF}} & \hlightPyellow{\text{NF}}~~+~~~\hlightPblue{\text{NSP}} & \hlightPred{\text{P}} & \hlightPred{\text{P}}~ +~~\hlightPblue{\text{NSP}} & \hlightPyellow{\text{NF}}~~+~~\hlightPgreen{\text{ST}} & \hlightPyellow{\text{NF}}~~+~~\hlightPblue{\text{NSP}}~~+~~\hlightPgreen{\text{ST}}  \\
    \midrule
    \multirow{3}{*}{CoNLL} & 5-shot & 0.535 \tiny{$\pm$ 0.030}& 0.614 \tiny{$\pm$ 0.057} & 0.584 \tiny{$\pm$ 0.056} & 0.609 \tiny{$\pm$ 0.040} & 0.567 \tiny{$\pm$ 0.025} & \textbf{0.654} \tiny{$\pm$ 0.044} \\
    & 10\% & 0.855 & 0.891 & 0.878 & 0.888 & 0.878 & \textbf{0.895} \\
    & 100\% & 0.919 & \textbf{0.92} & 0.911 & 0.915 & - & - \\
    \midrule
    \multirow{3}{*}{Onto} & 5-shot & 0.577 \tiny{$\pm$ 0.022} & 0.688 \tiny{$\pm$ 0.017} & 0.533 \tiny{$\pm$ 0.025} & 0.570 \tiny{$\pm$ 0.031} & 0.605 \tiny{$\pm$ 0.054} & \textbf{0.711} \tiny{$\pm$ 0.018} \\
    & 10\% & 0.861 & \textbf{0.869} & 0.854 & 0.846 & 0.867 & 0.867 \\
    & 100\% & 0.891 & 0.887 & 0.886 & 0.883 & - & - \\
    \midrule
    \multirow{3}{*}{WikiGold} & 5-shot & 0.470 \tiny{$\pm$ 0.065}& 0.640 \tiny{$\pm$ 0.042}& 0.511 \tiny{$\pm$ 0.064}& 0.604 \tiny{$\pm$ 0.054}& 0.481 \tiny{$\pm$ 0.091}& \textbf{0.684} \tiny{$\pm$ 0.032}\\
    & 10\% & 0.665 & 0.747 & 0.692 & 0.701 & 0.695 & \textbf{0.759} \\
    & 100\% & 0.807 & \textbf{0.839} & 0.801 & 0.827 & - & - \\
    \midrule
    \multirow{3}{*}{WNUT17} & 5-shot & 0.257 \tiny{$\pm$ 0.076}& 0.342 \tiny{$\pm$ 0.042}& 0.295 \tiny{$\pm$ 0.045} & 0.359 \tiny{$\pm$ 0.026} & 0.300 \tiny{$\pm$ 0.084} & \textbf{0.376} \tiny{$\pm$ 0.032}\\
    & 10\% & 0.483 & 0.492 & 0.485 & 0.478 & 0.490 & \textbf{0.505} \\
    & 100\% & 0.489 & 0.520 & 0.552 & \textbf{0.560} & - & - \\
    \midrule
    \multirow{3}{*}{MIT Movie} & 5-shot & 0.513 \tiny{$\pm$ 0.025}& 0.531 \tiny{$\pm$ 0.022}& 0.380 \tiny{$\pm$ 0.040}& 0.438 \tiny{$\pm$ 0.020}& 0.541 \tiny{$\pm$ 0.029}& \textbf{0.559} \tiny{$\pm$ 0.017}\\
    & 10\% & 0.651 & 0.657 & 0.563 & 0.583 & 0.659 & \textbf{0.666} \\
    & 100\% & \textbf{0.693} & 0.692 & 0.632 & 0.641 & - & - \\
    \midrule
    \multirow{3}{*}{MIT Restaurant} & 5-shot & 0.487 \tiny{$\pm$ 0.031} & 0.491 \tiny{$\pm$ 0.031} & 0.441 \tiny{$\pm$ 0.040} & 0.484 \tiny{$\pm$ 0.033} & 0.503 \tiny{$\pm$ 0.017} & \textbf{0.513} \tiny{$\pm$ 0.030}\\
    & 10\% & 0.745 & 0.734 & 0.713 & 0.721 & \textbf{0.750} & 0.741 \\
    & 100\% & 0.790 & \textbf{0.793} & 0.787 & 0.791 & - & - \\
    \midrule
    \multirow{3}{*}{SNIPS} & 5-shot & 0.792 \tiny{$\pm$ 0.014} & 0.824 \tiny{$\pm$ 0.018} & 0.750 \tiny{$\pm$ 0.025} & 0.773 \tiny{$\pm$ 0.021} & 0.796 \tiny{$\pm$ 0.016} & \textbf{0.830} \tiny{$\pm$ 0.016}\\
    & 10\% & 0.945 & \textbf{0.950} & 0.879 & 0.896  & 0.946 & 0.942 \\
    & 100\% & 0.970 & \textbf{0.972} & 0.923 & 0.956 & - & - \\
    \midrule
    \multirow{3}{*}{ATIS} & 5-shot & \textbf{0.908} \tiny{$\pm$ 0.007} & \textbf{0.908} \tiny{$\pm$ 0.008} & 0.842 \tiny{$\pm$ 0.026} & 0.896 \tiny{$\pm$ 0.009} & 0.904 \tiny{$\pm$ 0.010} & 0.905 \tiny{$\pm$ 0.012}\\
    & 10\% & 0.883 & \textbf{0.898} & 0.785 & 0.896 & & \\
    & 100\% & 0.953 & \textbf{0.956} & 0.929 & 0.943 & - & - \\
    \midrule
    \multirow{3}{*}{Multiwoz} & 5-shot & 0.123 \tiny{$\pm$ 0.083} & 0.198 \tiny{$\pm$ 0.031} & 0.219 \tiny{$\pm$ 0.032} & \textbf{0.451} \tiny{$\pm$ 0.023} & 0.200 \tiny{$\pm$ 0.082} & 0.225 \tiny{$\pm$ 0.042}\\
    & 10\% & 0.826 & 0.830 & 0.787 & 0.805 & 0.835 & \textbf{0.841} \\
    & 100\% & 0.880 & \textbf{0.885} &  0.837 & 0.845 & - & - \\
    \midrule
    \end{tabular}
    \caption{F1-score on unseen tasks not seen in training. \hlightPyellow{\text{NF}}~ is {\it naive fine-tuning} using a SoftMax objective, ~~\hlightPred{\text{P}}~ is {\it prototype-based training} using a nearest neighbor objective, ~~\hlightPblue{\text{NSP}}~ is {\it noising supervised pre-training} and ~~\hlightPgreen{\text{ST}}~ is {\it self-training}. \CL{Please consider to report the average results over all datasets} }
    \label{tab:unseen_tasks}
\end{table*}
